# Supplementary material for: Multimodal Task Vectors Enable Many-Shot Multimodal In-Context Learning
Source: arXiv:2406.15334 source file (2024-12-20)
Supplement: Supplementary file 1 [file 6_additional_sections.tex]

\section{Limitations}
\textbf{CCoT Template - To Be Edited}
In this work, we present a zero-shot Chain-of-Thought prompting method that utilizes scene-graph representations for multimodal and compositional visual reasoning tasks. We demonstrate improved performance on several different models and benchmarks. Nevertheless, our work has a central limitation. While extending context length is an active field of research, our method is limited by the current context lengths of the LLMs being used by the LMMs. Additionally, scene graphs are not particularly useful representations when performing multimodal tasks that emphasize language over visual reasoning, such as document understanding. Finally, we do not anticipate negative impacts of this work, but, as with any machine learning method, we recommend exercising caution.
